# Supplementary material for: The Satisfiability and Validity Problems for Probabilistic Computational Tree Logic are Highly Undecidable
Source: arXiv:2504.19207 source file (2025-04-30)
Supplement: Supplementary file 1 [file appendix.tex]

Here, we provide the proofs omitted in the main body of the paper due to space constraints.

\tausigma*
\begin{proof}
Recall that 
\begin{eqnarray*}
    I_q & = & \left(\frac{1-\sqrt{4q-3}}{2},  \frac{1+\sqrt{4q-3}}{2}\right)\\
    W   & = & I_q \times [0,\infty)\\
    \tau(\vec{v}) & = & \left( \frac{q{-}1{+}\vec{v}_1}{\vec{v}_1}, \frac{\vec{v}_2}{\vec{v}_1} \right)\\
    \sigma(\vec{v}) & = & \left( \frac{1{-}q}{1{-}\vec{v}_1}, \frac{\vec{v}_2(1{-}q)}{1{-}\vec{v}_1} \right) 
\end{eqnarray*}
%and $W =I_q \times (0,\infty)$.
\smallskip

\textit{Item~(a).}
Let $\vec{v} \in W$. We show that $\tau(\vec{v}) \in W$. Observe
\begin{eqnarray*}
   \tau(\vec{v})_1 & = & 1 - \frac{1-q}{\vec{v}_1}\\
     & < & 1 - \frac{2(1-q)}{1-\sqrt{4q-3}}\\
     & = & 1- \frac{(2-2q)}{1-\sqrt{4q-3}} \cdot \frac{1+\sqrt{4q-3}}{1+\sqrt{4q-3}}\\
     & = & 1- \frac{(2-2q)(1+\sqrt{4q-3})}{4-4q}\\
     & = & \frac{1+\sqrt{4q-3}}{2}
\end{eqnarray*}
Similarly, we obtain $\tau(\vec{v})_1 > \frac{1-\sqrt{4q-3}}{2}$, and hence $\tau(\vec{v})_1 \in I_q$. Since $\tau(\vec{v})_2 = \vec{v}_2/\vec{v}_1 > 0$, we have that $\tau(\vec{v}) \in W$ as required.

Now we show that $\sigma(\vec{v}) \in W$. Observe
\begin{eqnarray*}
    \sigma(\vec{v})_1 & = & \frac{1-q}{1-\vec{v}_1}\\
      & < & \frac{1-q}{1-\frac{1+\sqrt{4q-3}}{2}}\\[2ex]
      & = & \frac{2(1-q)}{1- \sqrt{4q-3}} \cdot \frac{1+\sqrt{4q-3}}{1+\sqrt{4q-3}}\\[2ex]
      & = & \frac{1+\sqrt{4q-3}}{2}
\end{eqnarray*}
Similarly, we obtain $\sigma(\vec{v})_1 >  \frac{1-\sqrt{4q-3}}{2}$. Since $\sigma(\vec{v})_2 = \frac{\vec{v}_2(1{-}q)}{1{-}\vec{v}_1} > 0$, we have that $\sigma(\vec{v}) \in W$.
\smallskip

\textit{Item~(b).}
Let $\vec{v} \in W$. Observe that $\tau(\vec{v})_1 > \vec{v}_1$ iff $(q{-}1{+}\vec{v}_1)/\vec{v}_1 > \vec{v}_1$ iff $\vec{v}_1^2 - \vec{v}_1 - q +1 < 0$ iff $\vec{v}_1 \in I_q$. This explains our choice of $I_q$. Furthermore, $\tau(\vec{v})_2 = \vec{v}_2/\vec{v}_1 \geq \vec{v}_2$; if $\vec{v}_2 > 0$, then $\tau(\vec{v})_2 > \vec{v}_2$.
\smallskip

\textit{Item~(c).} Let $\vec{v} \in W$. Observe
\begin{eqnarray*}
    \slope(\vec{u},\tau(\vec{v})) & = & \frac{\tau(\vec{v})_2}{\tau(\vec{v})_1 - \vec{v}_1} = \frac{\vec{v}_2}{q-1+\vec{v}_1(1 - \vec{v}_1)}
 \end{eqnarray*}
% \begin{eqnarray*}
%     \slope(\vec{v},\tau(\vec{v})) & = & \frac{\tau(\vec{v})_2 - \vec{v}_2}{\tau(\vec{v})_1 - \vec{v}_1} = \frac{\vec{v}_2(1-\vec{v}_1)}{q-1+\vec{v}_1(1 - \vec{v}_1)}
%  \end{eqnarray*}
 Similarly,
 \begin{eqnarray*}
    \slope(\tau(\vec{v}),\tau^2(\vec{v})) & = &  \frac{\tau(\vec{v})_2(1-\tau(\vec{v})_1)}{q-1+\tau(\vec{v})_1( 1 - \tau(\vec{v}_1))}\\[1ex]
    & = & \frac{\frac{\vec{v}_2}{\vec{v}_1}\left(1-\frac{q-1+\vec{v}_1}{\vec{v}_1}\right)}%
               {q-1 + \frac{q-1+\vec{v}_1}{\vec{v}_1} \left(1 - \frac{q-1+\vec{v}_1}{\vec{v}_1}\right)}\\[1ex]
    & = & \frac{\frac{\vec{v}_2}{\vec{v}_1}\left(\frac{1-q}{\vec{v}_1}\right)}%
    {q-1 + \frac{q-1+\vec{v}_1}{\vec{v}_1} \left(\frac{1-q}{\vec{v}_1}\right)}\\[1ex]  
    & = & \frac{\vec{v}_2}{q-1+\vec{v}_1(1-\vec{v}_1)}       
 \end{eqnarray*}
Hence, $\slope(\vec{u},\tau(\vec{v})) = \slope(\tau(\vec{v}),\tau^2(\vec{v}))$.
\smallskip

\textit{Item~(d).} Realize that 
\begin{eqnarray*}    
    \slope(\vec{u},\tau(\vec{u})) & = & \frac{y(1-\vec{v}_1)}{q-1+\vec{v}_1(1 - \vec{v}_1)}\\[1ex]
    \slope(\vec{v},\tau(\vec{v})) & = & \frac{\vec{v}_2(1-\vec{v}_1)}{q-1+\vec{v}_1(1 - \vec{v}_1)}
\end{eqnarray*}
SInce $0 \leq y < \vec{v}_2$, we have that $\slope(\vec{u},\tau(\vec{u})) < \slope(\vec{v},\tau(\vec{v}))$.

\smallskip

\textit{Item~(e).} It is trivial to verify that $\sigma(\tau(\vec{v})) = \tau(\sigma(\vec{v}) = \vec{v}$ for every $\vec{v} \in W$.
\end{proof}

\gproperties*
\begin{proof}
Let $\vec{v} \in W$. All claims follow directly from Lemma~\ref{lem-tausigma}. More concretely, for every $\vec{u} \in \Points(\vec{v})$, we have that both $\vec{u}$ and $L(\vec{u})$ are \emph{faces} of the convex set $\Area(\vec{v})$ (see, e.g., Section~2.6 in~\cite{Webster:book}), and the claims~(A) and~(B) are just instances of the defining property of a face. 
\end{proof}

\tauconvex*
\begin{proof}
It is easy to verify that for all $\vec{x},\vec{y} \in W$ and all $\lambda \in (0,1]$ we have that
\[
    \tau(\lambda\vec{x} + (1{-}\lambda)\vec{y}) \ = \ 
    \lambda'\tau(\vec{x}) + (1{-}\lambda') \tau(\vec{y})
\]
where 
\[
    \lambda' = \frac{\lambda \vec{x}_1}{\lambda\vec{x}_1 + (1{-}\lambda) \vec{y}_1} 
\]
Observe that $\lambda' \in (0,1]$. The lemma follows by putting $\vec{x} = \vec{w}$, $\vec{y} = \tau(\vec{w})$ and choosing $\lambda$ so that $\vec{u} = \lambda\vec{w} + (1{-}\lambda)\tau(\vec{w})$. 
\end{proof}  

\outlineseg*
\begin{proof}
First, we show that 
\begin{eqnarray}
    \lim_{k \to \infty} \sigma^k(\vec{\kappa})_1 & = & \frac{1-\sqrt{4q-3}}{2} \label{lim-2}
\end{eqnarray}
Let 
\[
    J_q =    \left[\frac{1-\sqrt{4q-3}}{2},  \vec{\kappa}_1\right] 
\]
By Lemma~\ref{lem-tausigma}, the infinite sequence  $\vec{\kappa}_1, \sigma(\vec{\kappa})_1, \sigma^2(\vec{\kappa})_1,\ldots$ is decreasing and bounded from below by $(1-\sqrt{4q-3})/2$. Consequently, the sequence has a limit~$\alpha \in J_q$, and hence it is also a Cauchy sequence, i.e.,
\[
    \lim_{k \to \infty} \sigma^{k+1}(\vec{\kappa})_1 - \sigma^{k}(\vec{\kappa})_1 = 0 \,.
\] 
Consider the function $f : J_q \to \R$ where 
\[
    f(x) \ = \ \frac{1-q-x(1-x)}{1-x}
\]
Observe that $f$ is non-negative and continuous. Furthermore, $f(x) = 0$ iff $x =  (1 - \sqrt{4q-3})/2$. Observe that for every $k \in \N$, we have that
\begin{eqnarray*}
    \sigma^{k+1}(\vec{\kappa})_1 - \sigma^{k}(\vec{\kappa})_1 \ = \ 
        f(\sigma^{k}(\vec{\kappa})_1) \,.
\end{eqnarray*}
Hence, 
\[
    0 \ = \ \lim_{k \to \infty} \sigma^{k+1}(\vec{\kappa})_1 - \sigma^{k}(\vec{\kappa})_1  =  \lim_{k \to \infty} f(\sigma^{k}(\vec{\kappa})_1) \ = \ f(\alpha)
\]
which implies $\alpha = (1 - \sqrt{4q-3})/2$.

Now let $\vec{v} \in W \smallsetminus \Area(\vec{\kappa})$ where $\vec{v}_1 \leq \vec{\kappa}_1$. By~\eqref{lim-2}, there exist $k \in \N$ such that $\sigma^k(\vec{\kappa})_1 \leq \vec{v}_1 < \sigma^{k-1}(\vec{\kappa})_1$. We put $\vec{u}_1 = \sigma^k(\vec{\kappa})_1$ and choose $\vec{u}_2$ so that 
\[
    \slope(\vec{u},\tau(\vec{u})) = \slope(\vec{u},\vec{v})\,.
\]
Hence, we require that
\[
     \frac{\vec{u}_2(1-\vec{u}_1)}{q-1+\vec{u}_1(1-\vec{u}_1)}    =
     \frac{\vec{v}_2 - \vec{u}_2}{\vec{v}_1 - \vec{u}_1}
\]
From this, we obtain
\[
    \vec{u}_2 = \frac{\vec{v}_2(q-1+\vec{u}_1(1-\vec{u}_1))}{\vec{v}_1 - \vec{u}_1 + q - 1 + \vec{u}_1(1-\vec{u}_1)}    
\]
and the proof is finished.
\end{proof}    

\Minskyproduct*
\begin{proof}
    Let $\M \equiv 1:\Ins_1;\cdots m: \Ins_m;$ be a non-deterministic two-counter Minsky machine. We start by transforming $\M$ into another two-counter Minsky machine $\widehat{\M}$ with $3m$ instructions constructed as follows:
    \begin{itemize}
        \item The first $m$ instructions of $\widehat{\M}$ are the same as the instructions of $\M$.
        %, except that all occurrences of $\textit{ goto } m{+}1$ are replaced with $\textit{ goto } 3m{+}1$.
        \item For every $j \in \{1,\ldots,m\}$, the machine $\widehat{M}$ contains the following labeled instructions:
        \begin{itemize}
            \item $\ \ m{+}j: \textit{if } c_1{=}0 \textit{ then goto } \{1\} \textit{ else dec } c_1; \textit{ goto } \{j\}$
            \item $2m{+}j: \textit{if } c_2{=}0 \textit{ then goto } \{1\} \textit{ else dec } c_2; \textit{ goto } \{j\}$
        \end{itemize}
        As we shall see, the target labels in the \textit{then} branches are insignificant and can be chosen arbitrarily.
        %\item The last instruction of $\widehat{M}$ is $3m{+}1 : \Halt$.
    \end{itemize}
    Observe that $\widehat{\M}$ has the same set of computations as $\M$, because the newly added instructions are not reachable from the initial configuration. Furthermore, if $\M$ is deterministic, then $\widehat{\M}$ is also deterministic.
    
    Let $L_1,L_2 \subseteq \{1,\ldots,3m\}$ be the sets of labels of all instructions of $\widehat{\M}$ operating on $c_1$ and $c_2$, respectively. Now, we construct two one-counter Minsky machines $\M_1,\M_2$ whose synchronized product simulates $\widehat{\M}$.
    
    Both $\M_1$ and $\M_2$ have $6m$ instructions. 
    % The instructions with labels $6m + 1$ and $6m+2$ are the same in $\M_1$ and $M_2$:
    % \begin{itemize}
    %     \item $6m+1 : \textit{if } c{=}0 \textit{ then goto 6m{+}2} \textit{ else dec } c; \textit{ goto } 6m{+}2$
    %     \item $6m+2 : \Halt$
    % \end{itemize}
    % As we shall see, the purpose $\Ins_{6m+1}$ is to ensure that both counters are zero when $\M_1 \times_I \M_2$ halts. 
    For notation convenience, the labels of $\M_1,\M_2$ are written as pairs $(\ell,0)$, $(\ell,+)$, where $\ell \in \{1,\ldots, 3m\}$.  
    
    For every $\ell \in \{1,\ldots, 3m\}$, the instructions labeled by $(\ell,0)$ and $(\ell,+)$ are constructed as follows: 
    Let $\Ins_\ell$ be the instruction of $\widehat{\M}$ with label $\ell$. If $\ell \in L_1$, then  
    \begin{itemize}
        \item $\M_1$ contains the instruction $(\ell,0): \overline{\Ins}$, where  $\overline{\Ins}$ is obtained from $\Ins_\ell$ as follows:
        \begin{itemize}
            \item $c_1$ is replaced with $c$;
            \item each set of target labels $L$ occurring in $\Ins_\ell$ is replaced with $\overline{L}$ obtained from $L$ by replacing every $u \in L$ with either $(u,+)$ or $(2m{+}u,0)$, depending on whether \mbox{$u \in L_1$} or $u \in L_2$, respectively.
        \end{itemize}
        \item $\M_2$ contains the instruction $(\ell,0): \textit{inc } c; \textit{goto } \{1\}$
        \item $\M_1$ contains the instruction $(\ell,+): \overline{\Ins}$, where  $\overline{\Ins}$ is obtained from $\Ins_\ell$ as follows:
        \begin{itemize}
            \item $c_1$ is replaced with $c$;
            \item each set of target labels $L$ occurring in $\Ins_\ell$ is replaced with $\overline{L}$ obtained from $L$ by replacing every $u \in L$ with $(u,0)$.
        \end{itemize}
        \item $\M_2$ contains the instruction\\ $(\ell,+): \textit{if } c{=}0 \textit{ then goto } \{1\} \textit{ else dec } c; \textit{ goto } \{1\}$ 
    \end{itemize}
    If $\ell \in L_2$, then 
    \begin{itemize}
        \item $\M_2$ contains the instruction $(\ell,0): \overline{\Ins}$, where  $\overline{\Ins}$ is obtained from $\Ins_\ell$ as follows:
        \begin{itemize}
            \item $c_2$ is replaced with $c$;
            \item each set of target labels $L$ occurring in $\Ins_\ell$ is replaced with $\overline{L}$ obtained from $L$ by replacing every $u \in L$ with either $(u,+)$ or $(m{+}u,0)$, depending on whether \mbox{$u \in L_2$} or $u \in L_1$, respectively.
        \end{itemize}
        \item $\M_1$ contains the instruction $(\ell,0): \textit{inc } c; \textit{goto } \{1\}$
        \item $\M_2$ contains the instruction $(\ell,+): \overline{\Ins}$, where  $\overline{\Ins}$ is obtained from $\Ins_\ell$ as follows:
        \begin{itemize}
            \item $c_2$ is replaced with $c$;
            \item each set of target labels $L$ occurring in $\Ins_\ell$ is replaced with $\overline{L}$ obtained from $L$ by replacing every $u \in L$ with $(u,0)$.
        \end{itemize}
        \item $\M_1$ contains the instruction\\ $(\ell,+): \textit{if } c{=}0 \textit{ then goto } \{1\} \textit{ else dec } c; \textit{ goto } \{1\}$ 
    \end{itemize}
    Furthermore, we put $I = (I_1,I_2)$, where $I_1$ is the set of all $(\ell,0),(\ell,+)$ such that $\ell \in L_1$, and $I_2$ contains the other labels. The computation of $\M_1 \times_I \M_2$ starts by executing the instructions with label $(1,0)$.
    
    Intuitively, $\M_1 \times_I \M_2$ simulates  $\widehat{\M}$ where the instructions on $c_1$ and $c_2$ are performed by $\M_1$ and $\M_2$, respectively.  
    As long as $\M_1$ performs instructions on $c_1$, $\M_2$ keeps incrementing/decrementing $c_2$ alternately (the flags $+$ and $0$ in the label indicate whether the ``inactive'' counter should be decremented or incremented; note that we only decrement the inactive counter when it was incremented before, and hence its value is certainly positive). When an instruction operating on $c_2$ is reached, the control is passed to $\M_2$. Before executing the instruction on $c_2$, $\M_2$ possibly decrements $c_2$ to restore its value. 
    It is easy to check that $\M$ is deterministic and bounded iff $\M_1 \times_I \M_2$ is deterministic and bounded, and $\M$ has a recurrent computation iff $\M_1 \times_I \M_2$ has a recurrent computation.

    %Recall that when $\widehat{M}$ halts, then both $c_1$ and $c_2$ are zero; the same holds for $\M_1 \times_I \M_2$. 
\end{proof}
